# Supplementary material for: Linguistic Characteristics of Censorable Language on SinaWeibo
Source: arXiv:1807.03654 source file (2018-07-10)
Supplement: Supplementary file 1 [file appendix1.pdf]

# Appendix I

### Control Questions of Crowdsourcing Experiments

请回答以下问题：

以下哪一句是通顺的句子？

- ○ 根据德国波恩大学发展研究中心的预算，全球人口将在同年增至98亿，到了2050年，全球粮食产量或会减少超过20%，但与此同时。
- ○ 根据德国波恩大学发展研究中心的预算，到了2050年，全球粮食产量或会减少超过20%，但与此同时，全球人口将在同年增至98亿。
- ○ 全球粮食产量或会减少超过20%，根据德国波恩大学发展研究中心的预算，但与此同时。全球人口将在同年增至98亿，到了2050年。。

请回答以下问题：

以下哪一个是成语无可奈何的意思？

- ○ 指感到没有办法，只有这样了
- ○ 指某一件事专心致志，顾不上睡觉，忘记了吃饭
- ○ 指心地单纯，没有做作和虚伪

请回答以下问题：

薄熙来犯了以下哪种罪行？

- ○ 偷窃
- ○ 贪污
- ○ 强奸

请回答以下问题：

以下哪个人物与薄熙来事件无关？

- ○ 王立军
- ○ 韩正
- ○ 谷开来

## CAP examples of Crowdsourcing Experiment from King et. al (2013)

**[反对政府; 提及的事件不涉及集体行动潜力]**
这是一个漠视生命的市政府[陕西省榆林市]、一个官员横行的市政府、一个没有公正的市政府，一个低级趣味的市政府，一个包二奶的市政府，一个为钱不要脸的市政府，一个为个权不要人格的市政府，一个没有血性的市政府，一个没有道德底线的市政府，一个出尔反尔的市政府，一个忘恩负义的市政府，一个不要子孙后代的市政府，一个什么怪事都出的市政府，一个什么的市政府，只要你想到的就有…

**[反對政府政策; 提及的事件不涉及集體行動潛力]**
我一直将中国近代史视为一场改良与革命的赛跑，在清末的大赛场上，最终革命跑到了头，改良的一切设计，在武昌起义枪声响起后成了废纸。中共的民主宪政承诺，是抗战结束前开出的远期支票，超过了一个甲子仍为兑现。当今中国社会缺乏诚信，要从毛泽东开始问责。邓小平在80年代提出的政治体制改革，在"8964" 事件后被长期搁置…近年所谓"党主立宪"之说，也是主流学者为维系一党执政地位所做的政治设计。

**[支持政府; 提及的事件涉及集体行动潜力：钱明奇抗争事件]**
爆炸案造成他本人和多名政府工作人员死亡的悲剧，即使钱明奇在微博里所称拆迁造成的个人损失是属实的，我们也应谴责他的极端报复行为…政府在连续出台保护被拆迁者利益的政策法规，媒体也在为公平对待被拆迁者大声疾呼，各地拆迁补偿上升速度，大多高于商品房售价上升速度，在不少地方，补偿款已经足以改变一个家庭的命运。

## Sample Questions of Crowdsourcing Experiment

以中国社会为背景，判断以下短文有否存在集体行动潜力：

> 【原济南书记王敏被曝与薄熙来熟识 曾关照薄家人】2013年薄熙来案在济南审理期间，薄熙来亲属抵达济南，被安排入住四星级宾馆舜耕山庄。舜耕山庄属济南市政府管理，是济南市委市政府的重要活动场地。据王敏朋友透露，王敏与薄熙来熟识多年，这一安排体现了王敏对薄家人的关照。

- ○ 有
- ○ 没有

以中国社会为背景，判断以下短文有否存在集体行动潜力：

> 当薄熙来在台上的时候，你反他，你错了。等薄倒台了，你还是错。周永康在台上的时候，你反他，你错了，等周倒台，你还是错。反过来，拥护薄周的人，什么时候都对，永远正确。

- ○ 有
- ○ 没有
